# Supplementary material for: Internet of Things Enabled Policing Processes
Source: arXiv:1908.09232 source file (2019-08-24)
Supplement: Supplementary file 1 [file chap_appendix.tex]

\chapter{Appendix}
\graphicspath{{ch_appendix/}}
